# Supplementary material for: Statistical modeling to adjust for time trends in adaptive platform trials utilizing non-concurrent controls
Source: arXiv:2403.14348 source file (2025-09-11)
Supplement: Supplementary file 1 [file Suppmaterial.pdf]

# Supplementary material for "Statistical modeling to adjust for time trends in adaptive platform trials utilizing non-concurrent controls"

Pavla Krotka[1], Martin Posch[1], Mohamed Gewily[2], Günter Höglinger[3,4,5,6], and Marta Bofill Roig*[1]

[1] *Center for Medical Data Science, Medical University of Vienna, Vienna 1090, Austria*
[2] *Department of Pharmacy, Uppsala University, Uppsala, Sweden.*
[3] *Department of Neurology, LMU University Hospital, Ludwig-Maximilians-Universität (LMU) München, Munich, Germany.*
[4] *German Center for Neurodegenerative Diseases (DZNE), Munich, Germany.*
[5] *Munich Cluster for Systems Neurology (SyNergy), Munich, Germany.*
[6] *Department of Neurology, Hannover Medical School, Hanover, Germany.*

## A Formal definition of the time variables

In this section, we present a formal definition of the considered periods, as well as units of calendar time in the platform trial.

We denote by $k$ ($k \in \{1, \dots, K\}$) the indicator of the experimental treatment arm, and by $s$ ($s \in \{1, \dots, S\}$) and $c$ ($c \in \{1, \dots, C\}$) the period and calendar time unit indicator, respectively. For each experimental treatment arm $k$ ($k \in \{1, \dots, K\}$), define $\mathbb{P}(k_j = k)$ as the probability that patient $j$ is allocated to this arm. This probability is strictly positive when the arm is active in the trial (i.e. open for randomization when patient $j$ is recruited) and 0 if the treatment arm is not yet or not anymore part of the platform, that is:

$$\mathbb{P}(k_j = k) = \begin{cases} \frac{1}{|\mathcal{K}_A(t_j)|+1} & \text{if } k \text{ is active} \\ 0 & \text{if } k \text{ is inactive} \end{cases}$$

where $\mathcal{K}_A(t) \subseteq \{1, \dots, K\}$ is the set of active experimental arms at time $t$. Note that formally, we say that treatment arm $k$ is active at time $t$ if $k \in \mathcal{K}_A(t)$ and inactive otherwise.

We define the entry and exit times of the treatment arm $k$ by $t_k^{entry}$ and $t_k^{exit}$ such that:

$$k \in \mathcal{K}_A(t) \text{ if and only if } t \in [t_k^{entry}, t_k^{exit}]$$

Denoting by $\mathbf{t}^{entry,exit} = \{t_1^{entry}, t_1^{exit}, t_2^{entry}, t_2^{exit}, \dots t_K^{entry}, t_K^{exit}\}$ a vector containing the entry and exit times of all experimental arms, we define the end of a period $s$ by $t_s^{end}$, considering:

$$t_1^{end} = \min\{t \in \mathbf{t}^{entry,exit} \mid t > 0\}$$
$$t_s^{end} = \min\{t \in \mathbf{t}^{entry,exit} \mid t > t_{s-1}^{end}\} \text{ for } s \in \{2, \dots, S\}$$

*marta.bofillroig@meduniwien.ac.at

where $S$ is the total number of periods in the trial as before.

Finally, the time interval for a period $s$ is given by:

$$T_1^S = [0, t_1^{end}]$$
$$T_s^S = (t_{s-1}^{end}, t_s^{end}] \text{ for } s \in \{2, \ldots, S\}$$

The trial can also be divided into equidistant units of calendar time. Given the length of the calendar time interval $c_{length}$, the trial consists of $C = \min\{x \in \mathbb{N} \mid x \geq t_S^{end}/c_{length}\}$ such intervals. The time interval for a calendar time unit $c$ is then given by:

$$T_1^C = [0, c_{length}] \text{ for } c = 1$$
$$T_c^C = ((c-1) \cdot c_{length}, c \cdot c_{length}] \text{ for } c \in \{2, \ldots, C-1\}$$
$$T_C^C = ((C-1) \cdot c_{length}, t_S^{end}] \text{ for } c = C$$

# B Further specification of the models for treatment-control comparisons

In this section, we provide technical details on the B-spline regression, as well as details on the structure of the covariance matrices in the mixed models with autocorrelated random effects.

## B.1 Spline regression

In the spline regression described in Section 2.2, we consider the B-spline function to model the time trend. This function is composed of multiple polynomial functions of a given degree $q$, which are joined together at points called *knots*, such that the entire spline is continuously differentiable up to the $(q-1)$th derivative [1].

In our case, the knots are placed within the range of the patient entry times $t_j$. To define a B-spline function, we first define the knot sequence

$$\zeta_1 = \ldots = \zeta_q = \zeta_{q+1} < \zeta_{q+2} < \ldots < \zeta_{q+Z+1} < \zeta_{q+Z+2} = \zeta_{q+Z+3} = \ldots = \zeta_{2q+Z+2}$$

where the $Z$ knots in the set $\{\zeta_{q+2}, \ldots, \zeta_{q+Z+1}\}$ are called *inner knots*, while $\zeta_{q+1}$ and $\zeta_{q+Z+2}$ are referred to as *boundary knots*. The additional knots $\{\zeta_1, \ldots, \zeta_q\}$, as well as $\{\zeta_{q+Z+3}, \ldots, \zeta_{Z+2q+2}\}$ are set equal to the boundary knots, even though their choice is essentially arbitrary and only needed because of the later recursive definition of the B-spline [2].

The function $f(t_j)$ can then be represented by a set of basis functions $B_i^q(t_j)$ as follows [3]:

$$f(t_j) = \sum_{i=1}^{q+Z+1} B_i^q(t_j)\beta_i$$

where $\beta_i$ are the associated regression coefficients and the functions $B_i^q(t_j)$ are defined using the following formula, recursive in $q$, as follows:

$$B_i^q(t_j) = \frac{t_j - \zeta_i}{\zeta_{i+q} - \zeta_i} B_i^{q-1}(t_j) + \frac{\zeta_{i+q+1} - t_j}{\zeta_{i+q+1} - \zeta_{i+1}} B_{i+1}^{q-1}(t_j), \qquad i = 1, \dots, q + Z + 1$$

with

$$B_i^0 = \begin{cases} 1 & \zeta_i \leq t_j < \zeta_{i+1} \\ 0 & \text{otherwise} \end{cases}$$

and

$$B_i^0 \equiv 0 \text{ if } \zeta_i = \zeta_{i+1}$$

As described in the main paper, we evaluate two strategies for the positions of the inner knots $\{\zeta_{q+2}, \dots, \zeta_{q+Z+1}\}$. Firstly, we place the inner knots to the beginning of each period $s = 2, \dots, S$, such that one polynomial of degree $q$ is always fitted to each period. In this case, the number of inner knots $Z = S - 1$. Moreover, we consider placing the inner knots equidistantly, according to the length of the calendar time unit, and thus fitting a polynomial of degree $q$ to each calendar time interval, which leads to $Z = C - 1$. The boundary knots $\zeta_{q+1}$ and $\zeta_{q+K+2}$ are always set to 1 and $N$, respectively, hence to the beginning and end of the trial.

## B.2 Mixed-effect models with autocorrelated random effects

In the mixed-effect models with autocorrelated random effects, described in Section 2.3, the random effects $u_s$ for individual periods are assumed to follow a normal distribution with mean 0, constant variance $\sigma^2_{period}$ and an AR(1) correlation structure, i.e.:

$$\boldsymbol{u} \sim \mathcal{N}(0, \sigma^2_{period} \cdot \Sigma_{S_M \times S_M})$$

$$\Sigma_{S_M \times S_M} = \begin{bmatrix} 1 & \phi & \cdots & \phi^{S_M-1} \\ \phi & 1 & \cdots & \phi^{S_M-2} \\ \vdots & \vdots & \ddots & \vdots \\ \phi^{S_M-1} & \phi^{S_M-2} & \cdots & 1 \end{bmatrix}$$

An analogous distribution is assumed for the random effects $u_c$ associated with different calendar times:

$$\boldsymbol{u} \sim \mathcal{N}(0, \sigma^2_{calendar} \cdot \Sigma_{C_M \times C_M})$$

$$\Sigma_{C_M \times C_M} = \begin{bmatrix} 1 & \phi & \cdots & \phi^{C_M-1} \\ \phi & 1 & \cdots & \phi^{C_M-2} \\ \vdots & \vdots & \ddots & \vdots \\ \phi^{C_M-1} & \phi^{C_M-2} & \cdots & 1 \end{bmatrix}$$

The parameter $\phi$ denotes the correlation between two adjacent periods or calendar time units. Note that $\phi$ can range from -1 to 1 and the correlation of periods that are $w$ units apart is equal to $\phi^w$, such that the correlation is weaker for periods or calendar time units that are further apart.

# C Additional Results

**Figure S1: Setting 1A:** Type I error rate and power of the fixed effect regression model with period adjustment compared to the pooled and separate analyses with respect to the strength of the time trend $\lambda$. In this example, $d = 400$ and $n = 250$ in each experimental arm and a linear shape of the time trend are used. Results for different experimental arms are shown in the rows.

**Figure S2: Setting 1A:** Type I error rate and power of the fixed effect regression model with period adjustment compared to the pooled and separate analyses with respect to the timing of adding the treatment arms. In this example, $n = 250$ in each experimental arm and a linear time trend with strength $\lambda = 0.5$ are considered. Results for different experimental arms are shown in the rows.

**Figure S3: Setting 1A:** Type I error rate and power of the regression model with period adjustment compared to the pooled and separate analyses with respect to the index of the evaluated arm. Here, $d = 200$, $n = 250$ in each experimental arm, and a linear time trend with strength $\lambda = 0.5$ are considered.

**Figure S4: Setting 1B:** Type I error rate and power for the spline regression model with knots according to periods or calendar time units compared to the regression model with period adjustment with respect to the strength of the time trend $\lambda$ using different time trend patterns. In this example, $n = 250$ in each experimental arm and $N_p = 1660$ in case of inverted-U trend (corresponding to the middle of the trial) are used. In case of calendar time adjustment, unit size of 100 patients is considered. Treatment arm 5 is being evaluated. Results for different degrees of the polynomial spline (linear, quadratic, cubic) are shown in the rows.

**Figure S5: Setting 1B:** Type I error rate and power for the cubic spline regression model with knots according to periods or calendar time units compared to the regression model with period adjustment with respect to the strength of the time trend $\lambda$ using different time trend patterns. In this example, $n = 250$ in each experimental arm, $N_p = 1660$ in case of inverted-U trend (corresponding to the middle of the trial) are used. In case of calendar time adjustment, unit size of 100 patients is considered. Results for different experimental arms are shown in the rows.

**Figure S6: Setting 2A:** Type I error rate and power of the regression model with calendar time adjustment compared to the regression model with period adjustment and separate analysis with respect to the size of the calendar time unit under different time trend patterns. In this example, $n = 250$ in each experimental arm, $\lambda = 0.125$ and $N_p = 750$ in case of inverted-U trend (corresponding approximately to the middle of the trial) are considered. Results for different experimental arms are shown in the rows.

**Figure S7: Setting 2A:** Type I error rate and power of the regression model with calendar time adjustment compared to the regression model with period adjustment and separate analysis with respect to the strength of the time trend $\lambda$ under different time trend patterns. In this example, $n = 250$ in each experimental arm, $N_p = 750$ in case of inverted-U trend (corresponding approximately to the middle of the trial) and calendar time unit size of 100 are used. Results for different experimental arms are shown in the rows.

**Figure S8: Setting 2B:** Type I error rate and power of the mixed model with period and calendar time

adjustments as uncorrelated and autocorrelated random effects, compared to the fixed effect regression model with period adjustment with respect to the pattern and strength of the time trend. Sample sizes of $n = 250$ in each experimental arm, $N_p = 750$ in case of inverted-U trend (corresponding approximately to the middle of the trial) are used. In case of calendar time adjustment, unit size of 100 patients is considered. Results for different experimental arms are shown in the rows.

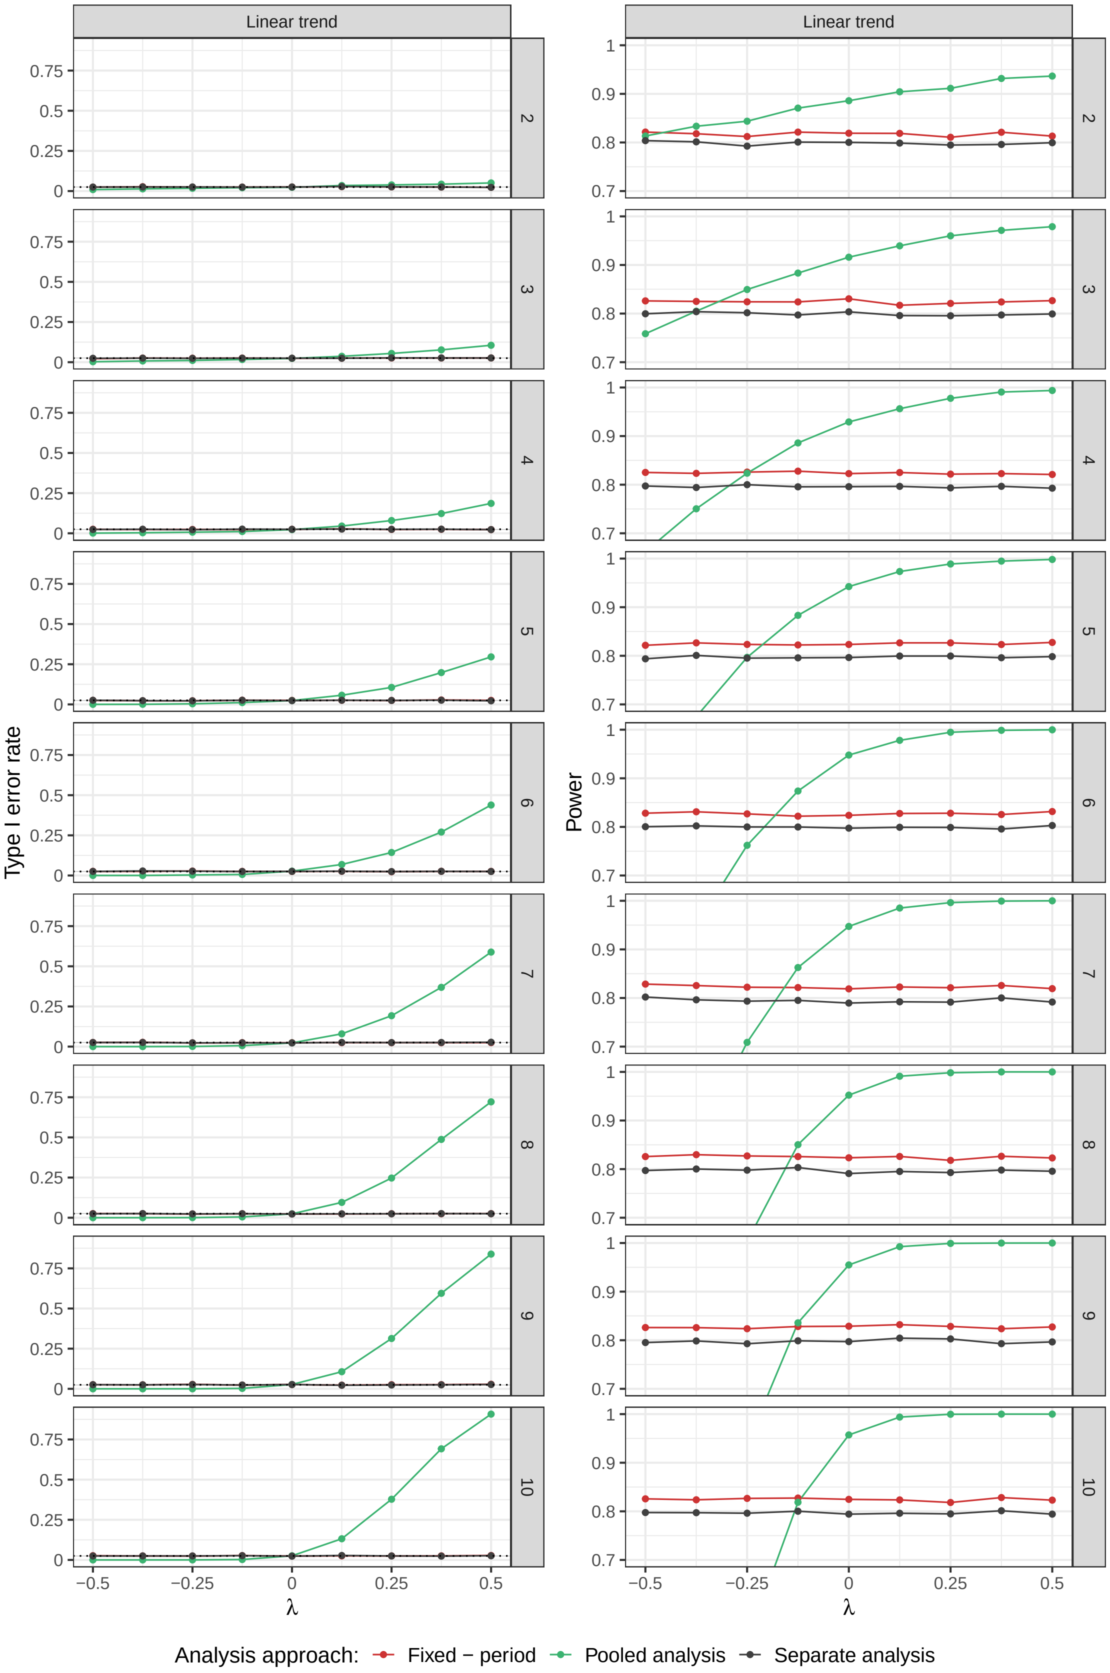
Linear trend
Linear trend
Type I error rate
Power
λ
λ
2
3
4
5
6
7
8
9
10
Analysis approach: Fixed − period Pooled analysis Separate analysis

Figure S1

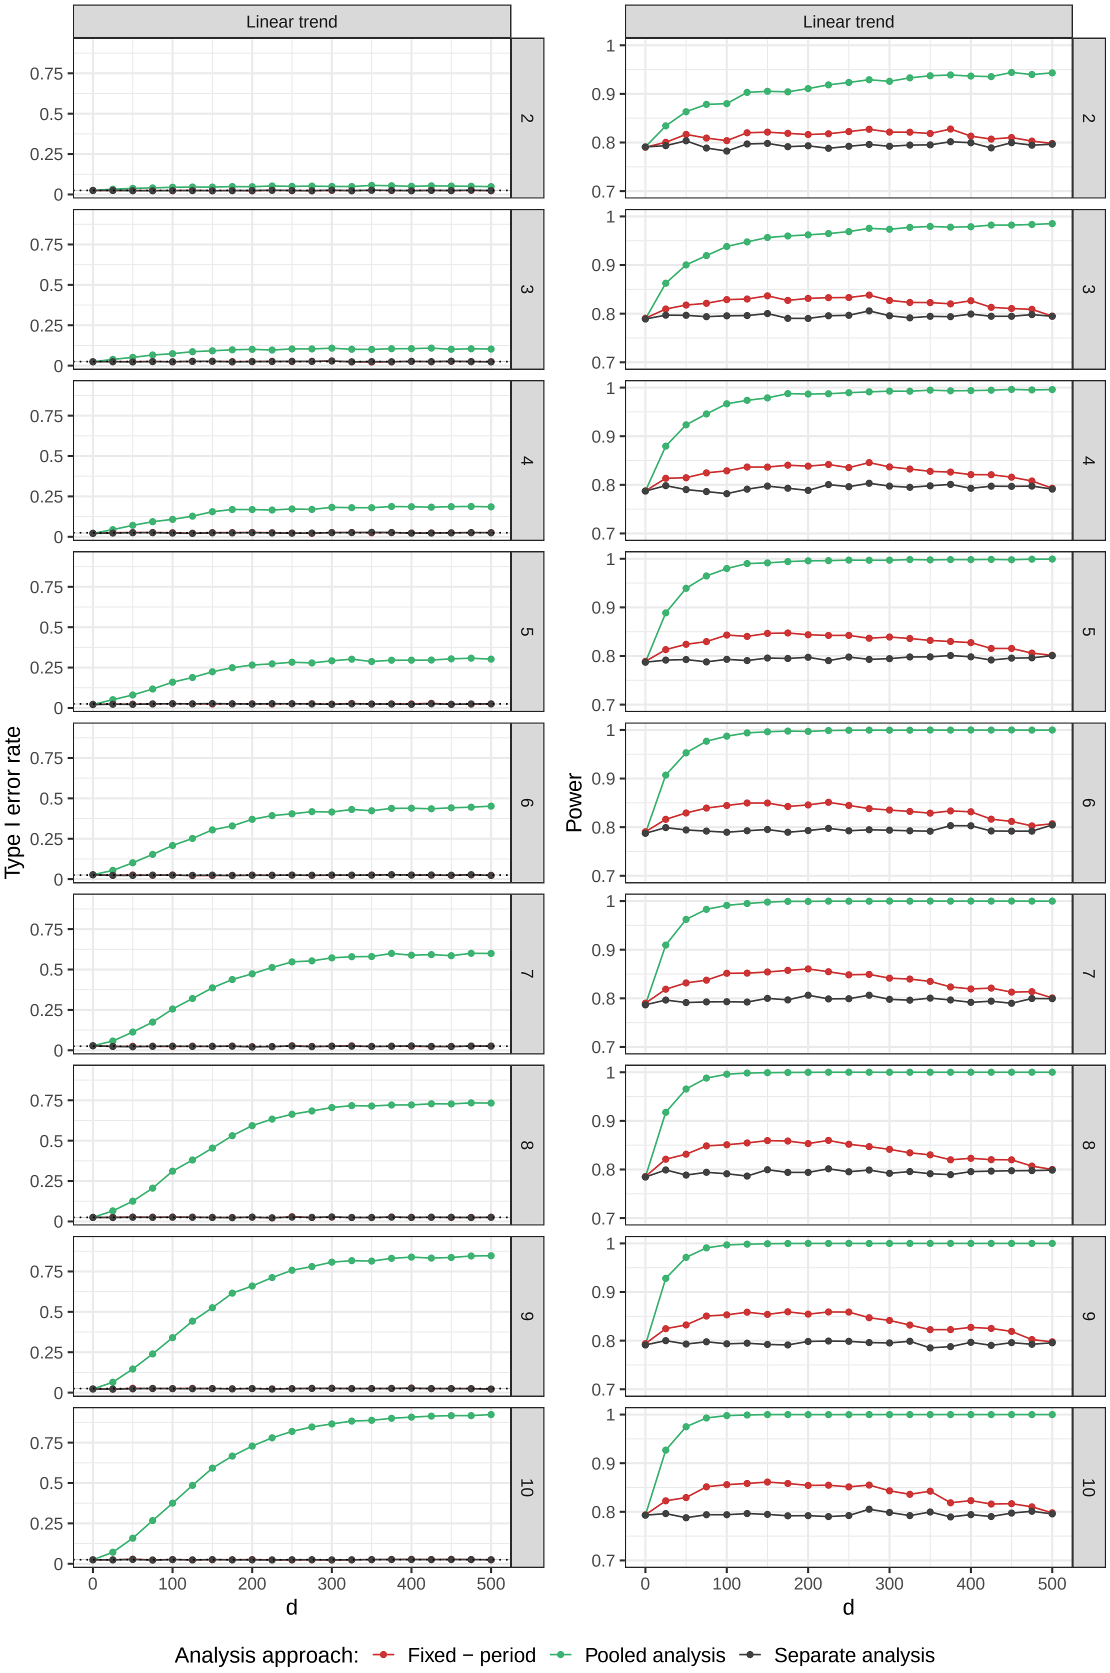
Linear trend
Linear trend
Type I error rate
Power
d
d
Analysis approach: Fixed − period Pooled analysis Separate analysis

Figure S2

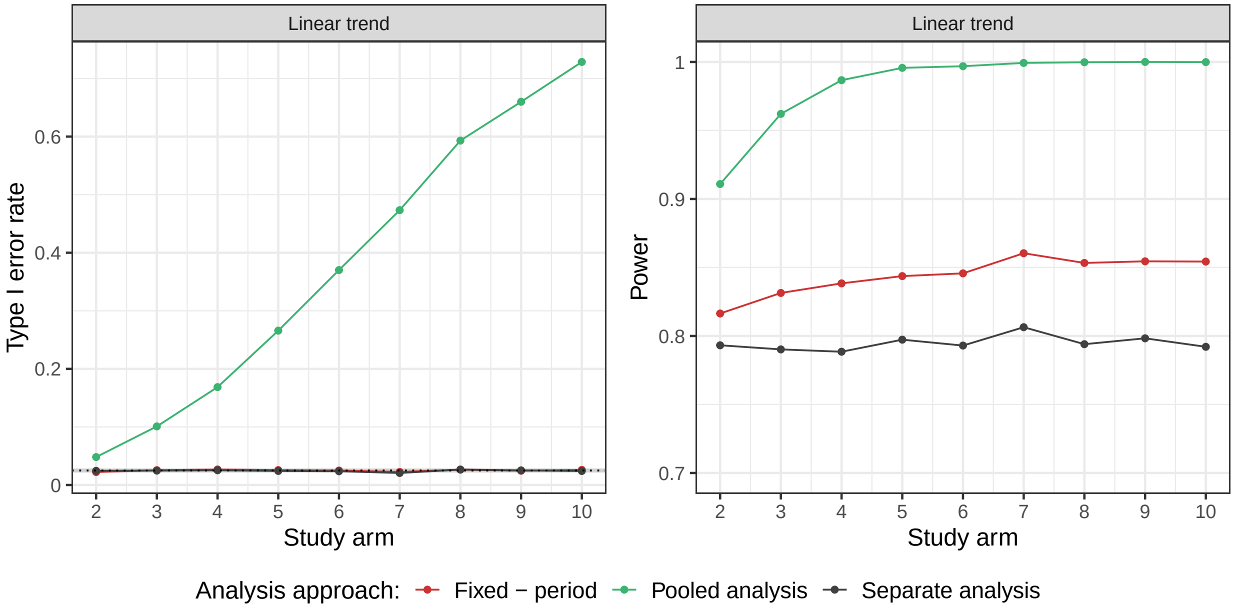
Linear trend
Type I error rate
0.6
0.4
0.2
0
2 3 4 5 6 7 8 9 10
Study arm
Linear trend
Power
1
0.9
0.8
0.7
2 3 4 5 6 7 8 9 10
Study arm
Analysis approach: Fixed − period Pooled analysis Separate analysis

Figure S3

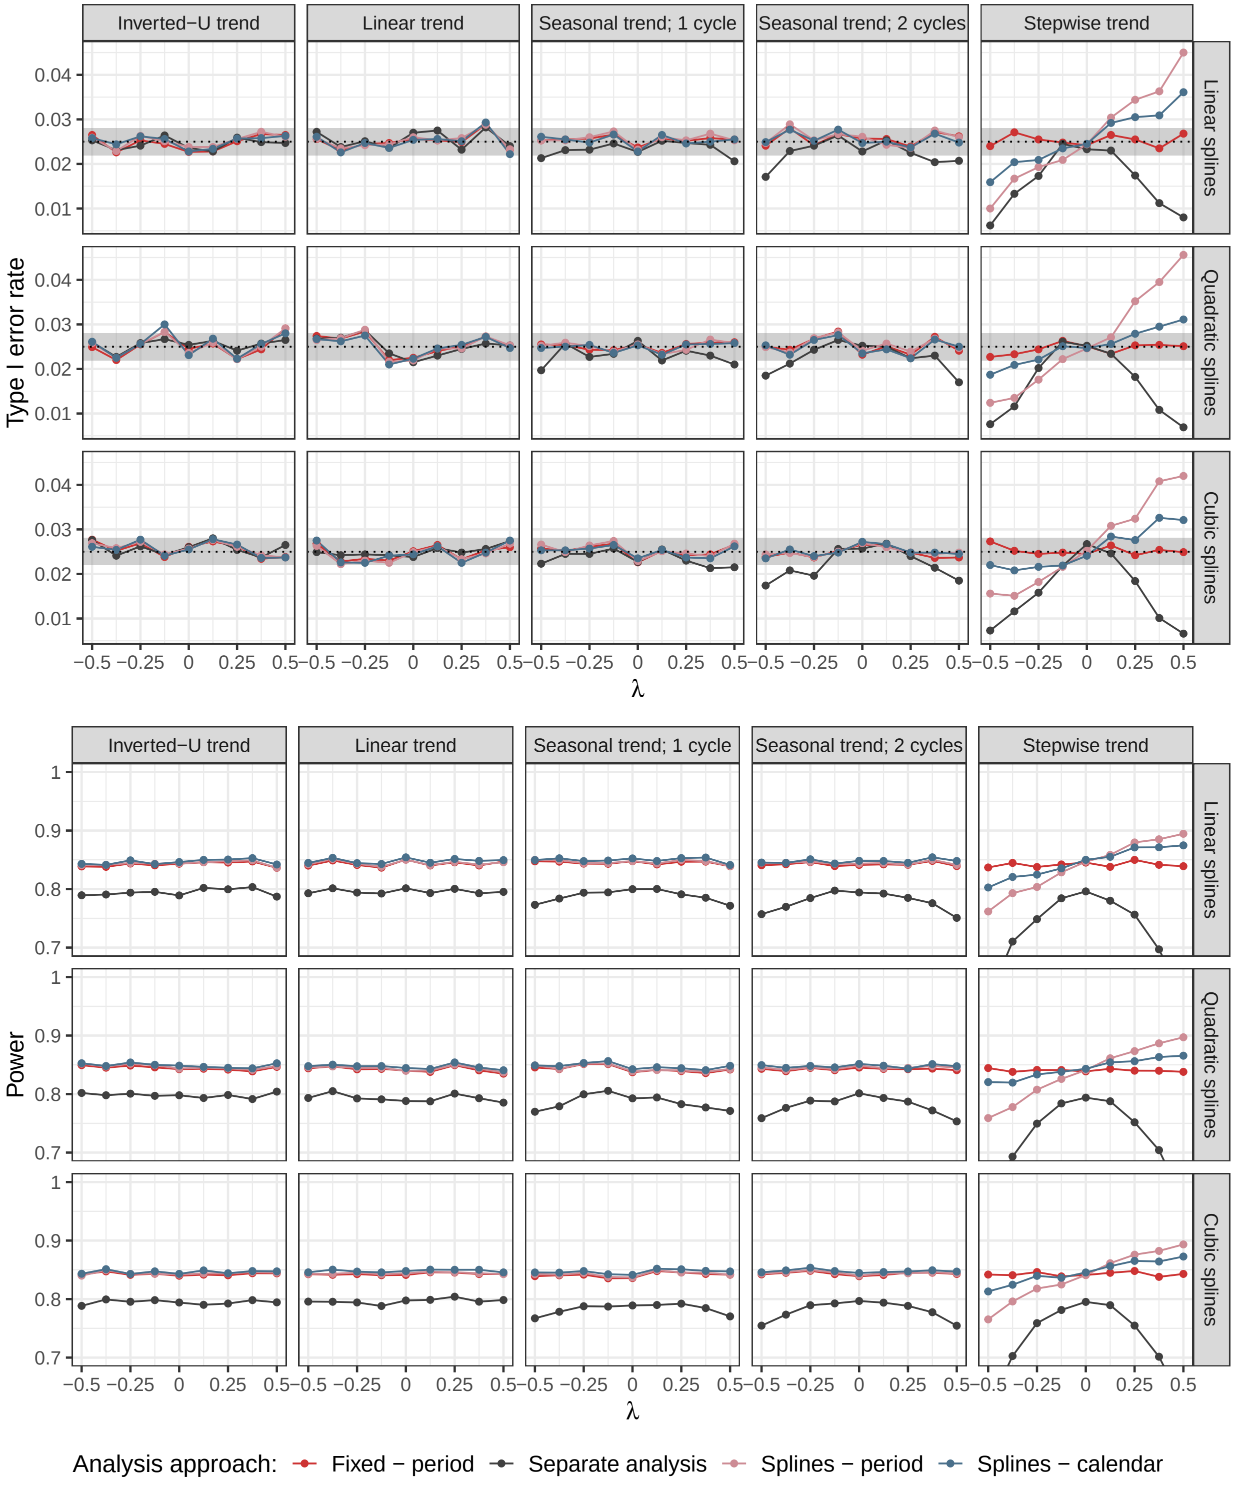
Inverted−U trend
Linear trend
Seasonal trend; 1 cycle
Seasonal trend; 2 cycles
Stepwise trend
Linear splines
Quadratic splines
Cubic splines
Type I error rate
Power
λ
Analysis approach: Fixed − period Separate analysis Splines − period Splines − calendar

Figure S4

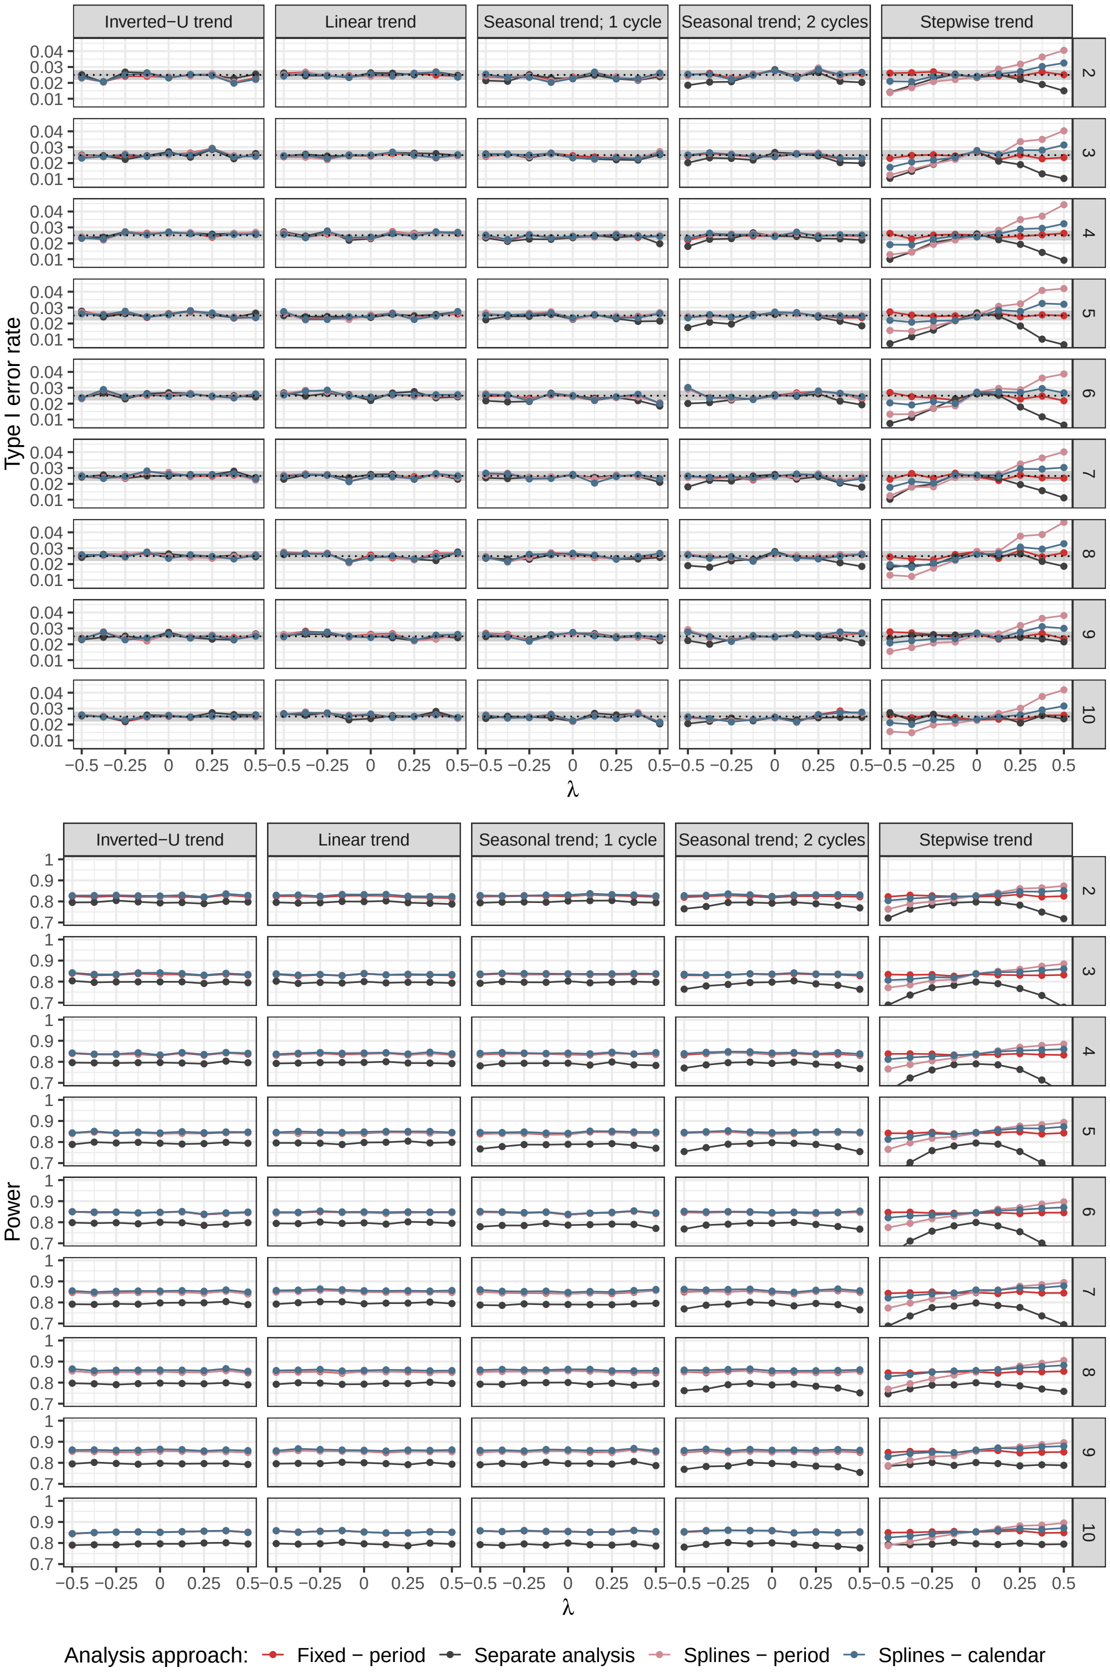
Inverted−U trend
Linear trend
Seasonal trend; 1 cycle
Seasonal trend; 2 cycles
Stepwise trend
Type I error rate
Power
λ
2
3
4
5
6
7
8
9
10
Analysis approach: Fixed − period Separate analysis Splines − period Splines − calendar

Figure S5

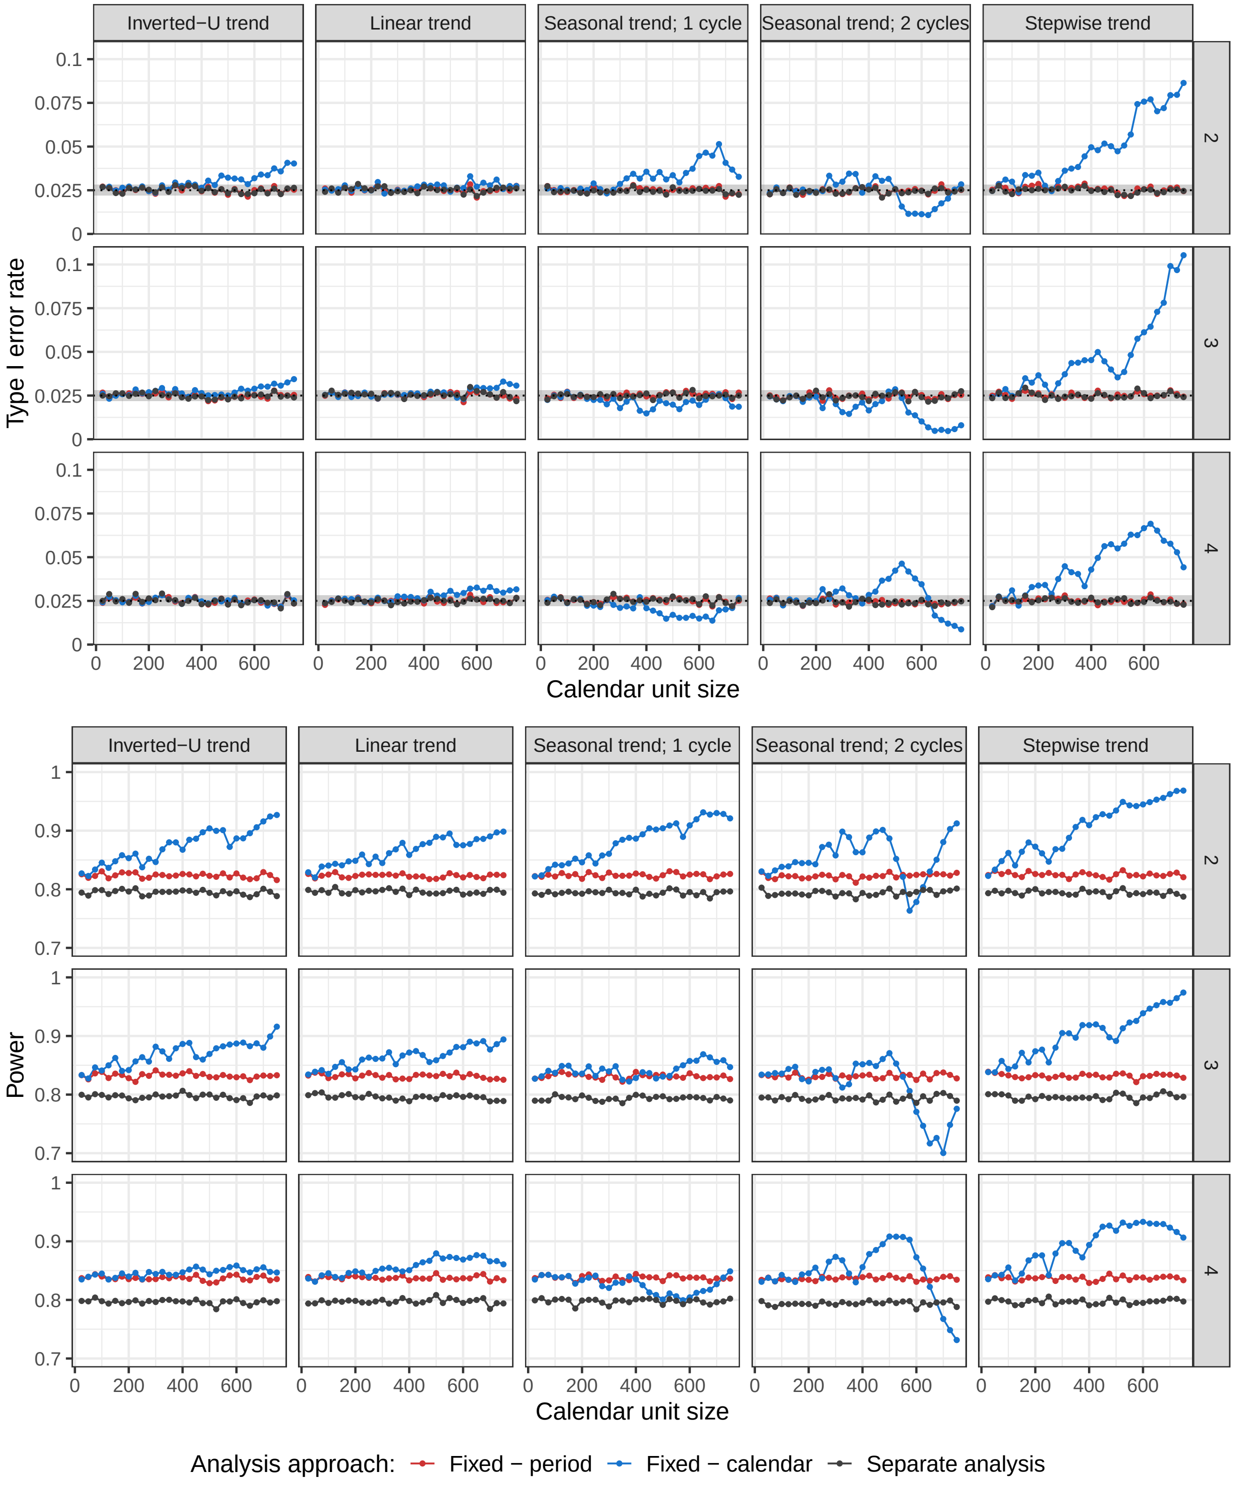
Inverted−U trend
Linear trend
Seasonal trend; 1 cycle
Seasonal trend; 2 cycles
Stepwise trend
Type I error rate
0.1
0.075
0.05
0.025
0
2
3
4
0
200
400
600
Calendar unit size
Power
1
0.9
0.8
0.7
Analysis approach:
Fixed − period
Fixed − calendar
Separate analysis

Figure S6

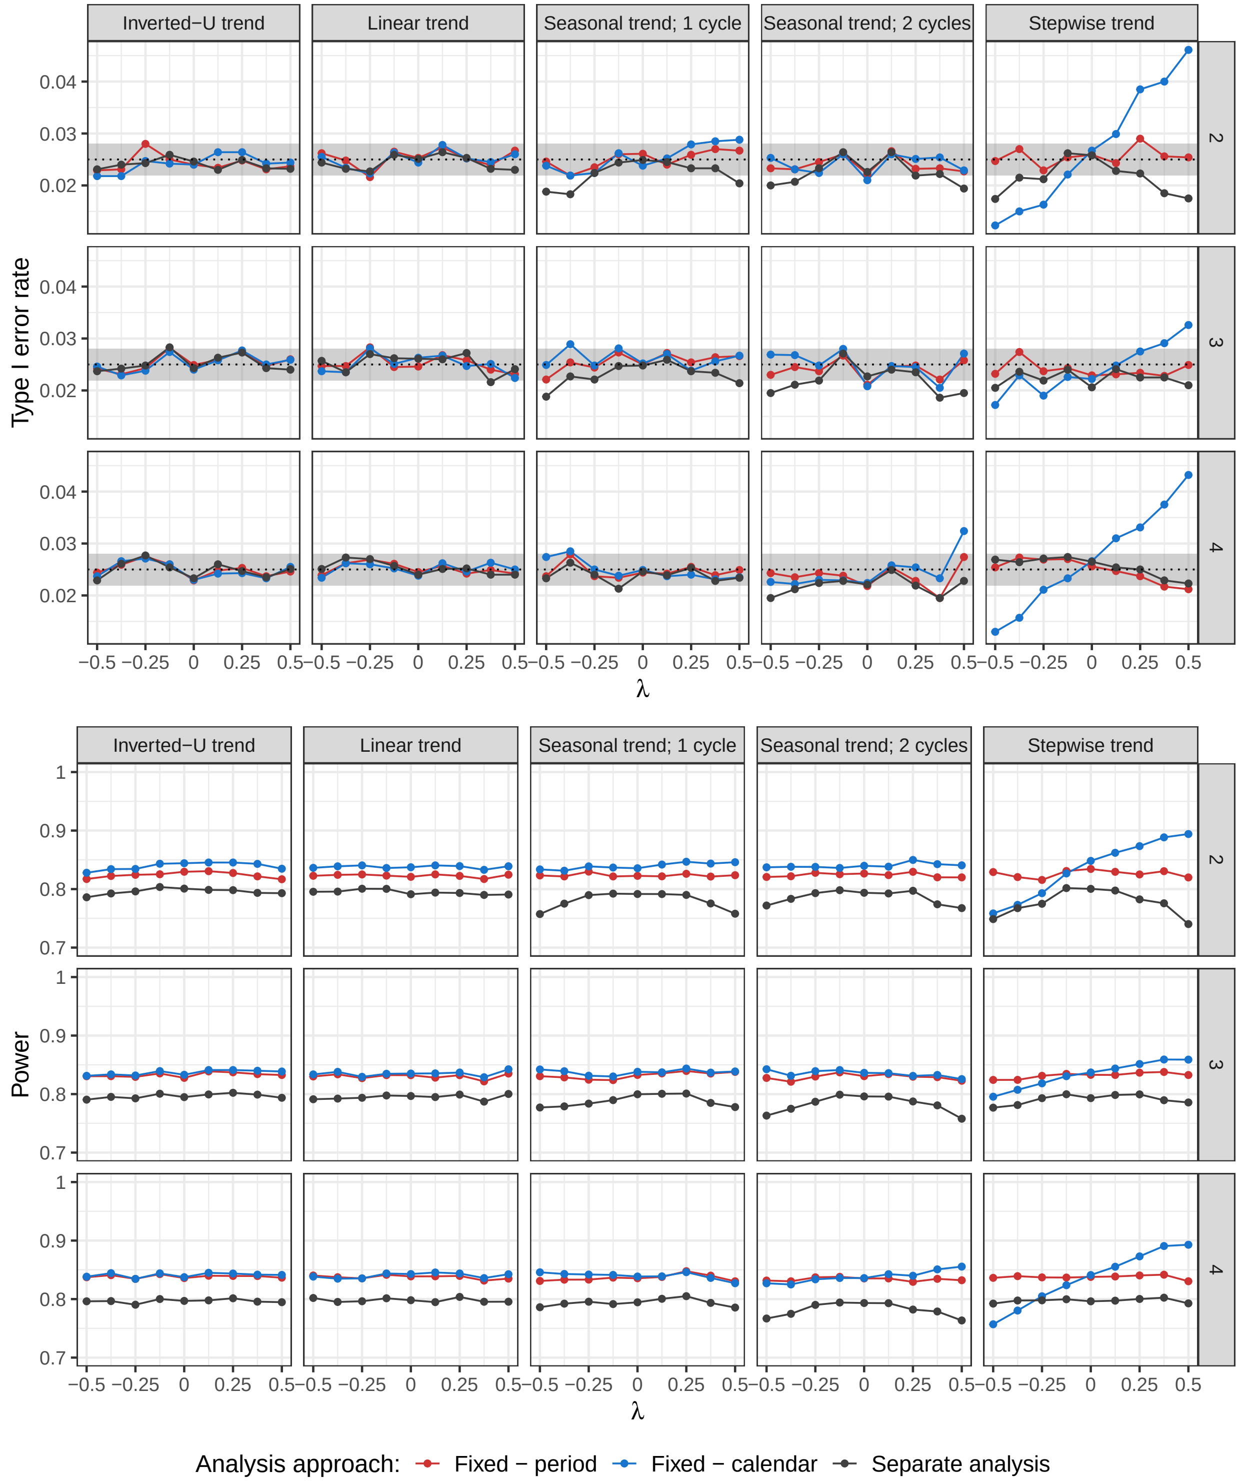
Inverted−U trend
Linear trend
Seasonal trend; 1 cycle
Seasonal trend; 2 cycles
Stepwise trend
Type I error rate
Power
λ
Analysis approach: Fixed − period Fixed − calendar Separate analysis

Figure S7

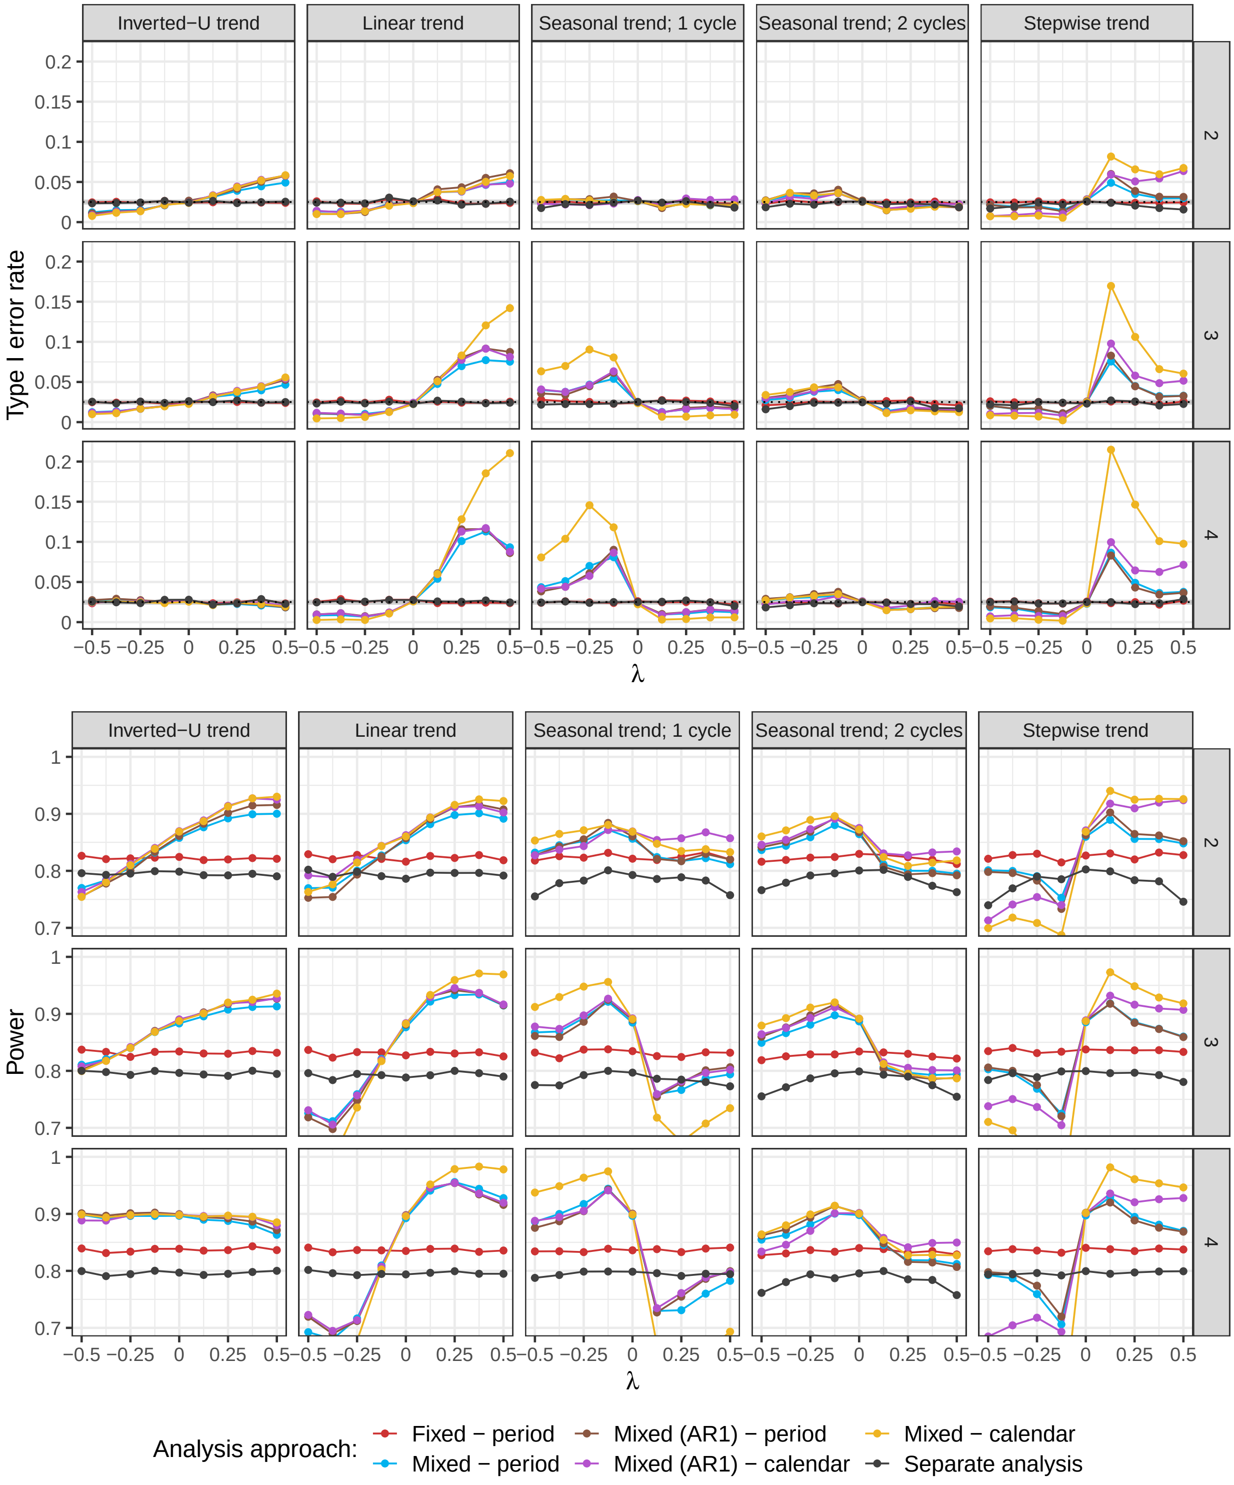
Inverted−U trend
Linear trend
Seasonal trend; 1 cycle
Seasonal trend; 2 cycles
Stepwise trend
Type I error rate
Power
2
3
4
λ
Analysis approach:
Fixed − period
Mixed − period
Mixed (AR1) − period
Mixed (AR1) − calendar
Mixed − calendar
Separate analysis

Figure S8

# References

[1] Paul H.C. Eilers and Brian D. Marx. Flexible smoothing with B-splines and penalties. *Statistical Science*, 11(2):89–121, 1996.

[2] Aris Perperoglou, Willi Sauerbrei, Michal Abrahamowicz, and Matthias Schmid. A review of spline function procedures in R. *BMC Medical Research Methodology*, 19(1):1–16, 2019.

[3] Simon N. Wood. *Generalized Additive Models: An Introduction with R*. Chapman and Hall/CRC, 2017.
